# Supplementary material for: KAT-Coder Technical Report
Source: arXiv:2510.18779 source file (2025-10-31)
Supplement: Supplementary file 1 [file appendix.tex]

\section{Appendix}
